# Supplementary material for: Intrinsically motivated graph exploration using network theories of human curiosity
Source: arXiv:2307.04962 ancillary file (2023-12-01)
Supplement: Supplementary file 1 [file Supplement.pdf]

# Supplement: Intrinsically Motivated Graph Exploration Using Network Theories of Human Curiosity

## Contents

**S1 Synthetic graph models** **S2**

**S2 Training and validation curves** **S4**

**S3 Atlases** **S6**

**S4 Trajectory length and network size generalization** **S7**

**S5 Real-world graph datasets** **S11**

**S6 Random walker diffusion** **S12**

**S7 Human trajectories of graph exploration** **S13**

**S8 Training details** **S14**
S8.1 Hyperparameters . . . . . . . . . . . . . . . . . . . . . . . . . . . . . . . . . . . . . S14
S8.2 Algorithm . . . . . . . . . . . . . . . . . . . . . . . . . . . . . . . . . . . . . . . . . S15

**S9 Citation diversity statement** **S16**

**S10References** **S17**

## S1 Synthetic graph models

We evaluate the performance of GNN-based exploration agents in environments generated by four different types of synthetic graph models:

- Random geometric (RG): Graph-structured environments, such as transportation networks or power grids, are embedded in physical space. Random geometric graphs model such environments by placing nodes within a unit cube of chosen dimensionality. The model places nodes uniformly at random inside the cube. An edge connects a pair of nodes if the distance between the nodes is less than or equal to a radius value. For a 2-dimensional space, we set the radius value to $0.25$.
- Watts-Strogatz (WS): Many real-world networks possess a "small-world" topology, whereby distant nodes can be reached by a small number of hops from any node in the graph. The WS model creates graphs with a small-world topology by creating a ring graph and adding edges from each node to its $k$ nearest neighbors. Each edge is then rewired at random with probability $p$. We set $k = 4$ and $p = 0.1$.
- Barabási-Albert (BA): Starting with a randomly connected skeleton of $m$ nodes, the BA model, also known as the preferential attachment model, adds nodes sequentially. Each new node is connected to $m$ existing nodes with a probability proportional to node degree. This "rich-gets-richer" growth scheme results in graphs with heavy-tailed degree distributions. We set $m = 4$.
- Erdös-Rényi (ER): The ER model produces random graphs by adding edges between nodes with probability $p$. We set $p = 0.2$.

We depict representative networks for each graph model in Figure S1.

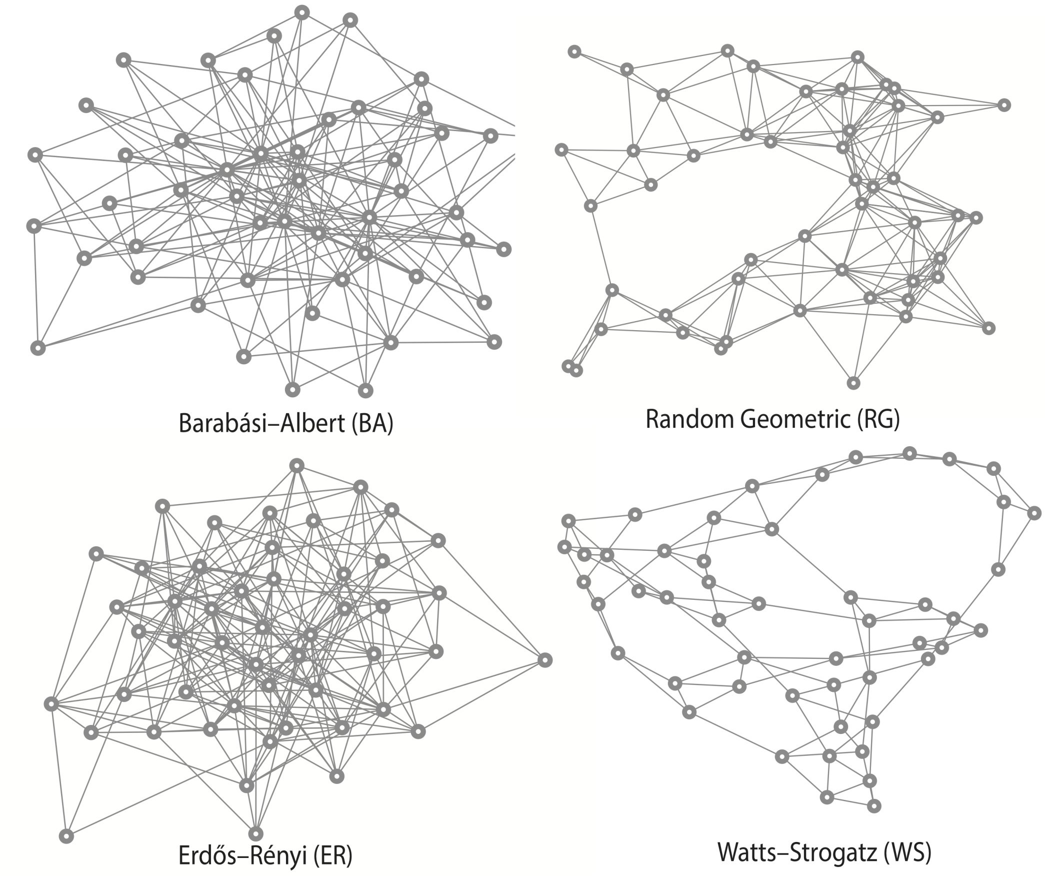


Figure S1: **Synthetic graph models.** Examples of synthetic graph environments. From left to right, top to bottom: (a) Barabási-Albert graph, (b) random geometric graph, (c) Erdös-Rényi graph, and (d) Watts-Strogatz graph. Each graph comprises 50 nodes. Other hyperparameters for the generative processes are described in the main text.

Each model leads to distinct graph properties, allowing us to test training and generalization performance for a variety of graph topologies. Figure S1 depicts example networks for each of the four network types. The BA model relies on preferential attachment, resulting in a scale-free degree distribution with few very highly connected nodes. The RG model embeds nodes in physical space. The ER model generates random connections between nodes based on a specified probability, leading to a uniform degree distribution. Lastly, the WS model starts with a regular lattice-like structure and introduces random rewiring, resulting in a small-world topology with local clustering and short average path lengths. Code to generate graphs from each of the four models has been attached to this submission.

# S2 Training and validation curves

Next, we plot the training and testing performance of the GNN agents in different synthetic graph environments while optimizing for information gap theory (Figure S2) and compression progress theory (Figure S3). We depict the average total reward, or the return, gathered by each agent in 100 training and 10 testing environments. We evaluate after every 100 training episodes. During each testing instance, results are averaged across 10 episodes in each of the 10 environments. The figures demonstrate that the GNNs train successfully as well as generalize when optimizing for information gaps and network compressibility.

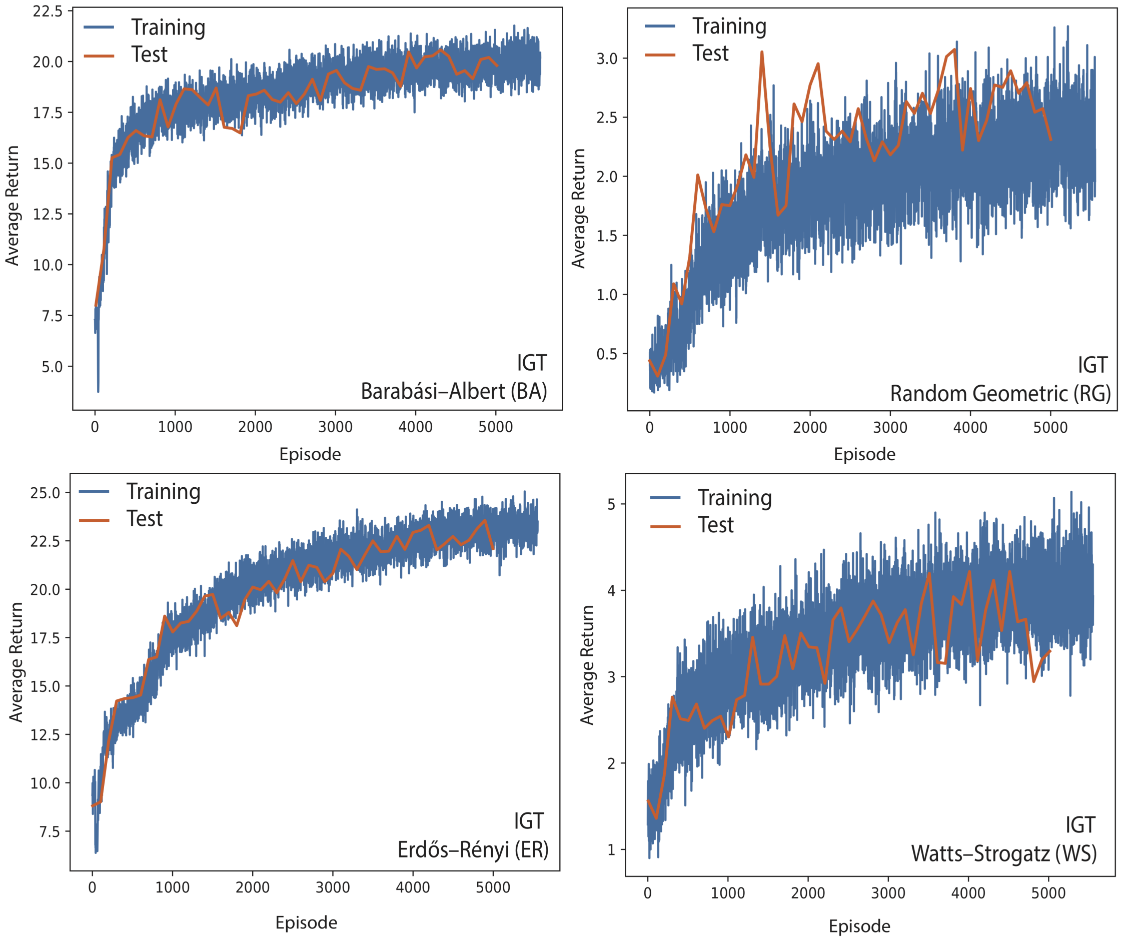


Figure S2: **Training and validation curves for information gap theory.** We plot the training and validation performances of GNNs trained to optimize for topological gaps. Performance is measured as the average return. From left to right, top to bottom: (a) BA graphs, (b) RG graphs, (c) ER graphs, and (d) WS graphs. The results demonstrate generalization to the test set across several graph topologies.

Compared to the information gap theory, training converges faster when optimizing for network compressibility. The return values tend to plateau resulting in diminishing marginal gains with increased training.

Notably, the IGT agents learn noisily in the random geometric and Watts-Strogatz graph environments. This can be attributed to the high local organization present in both types of graphs, as depicted in Figure S1. These topologies likely make it difficult early on for an agent to build topological cavities in a small number of steps. However, it is also worth noting that despite the quicker convergence in the CPT agents relative to the IGT agents, the IGT agents outperform other exploration baselines consistently.

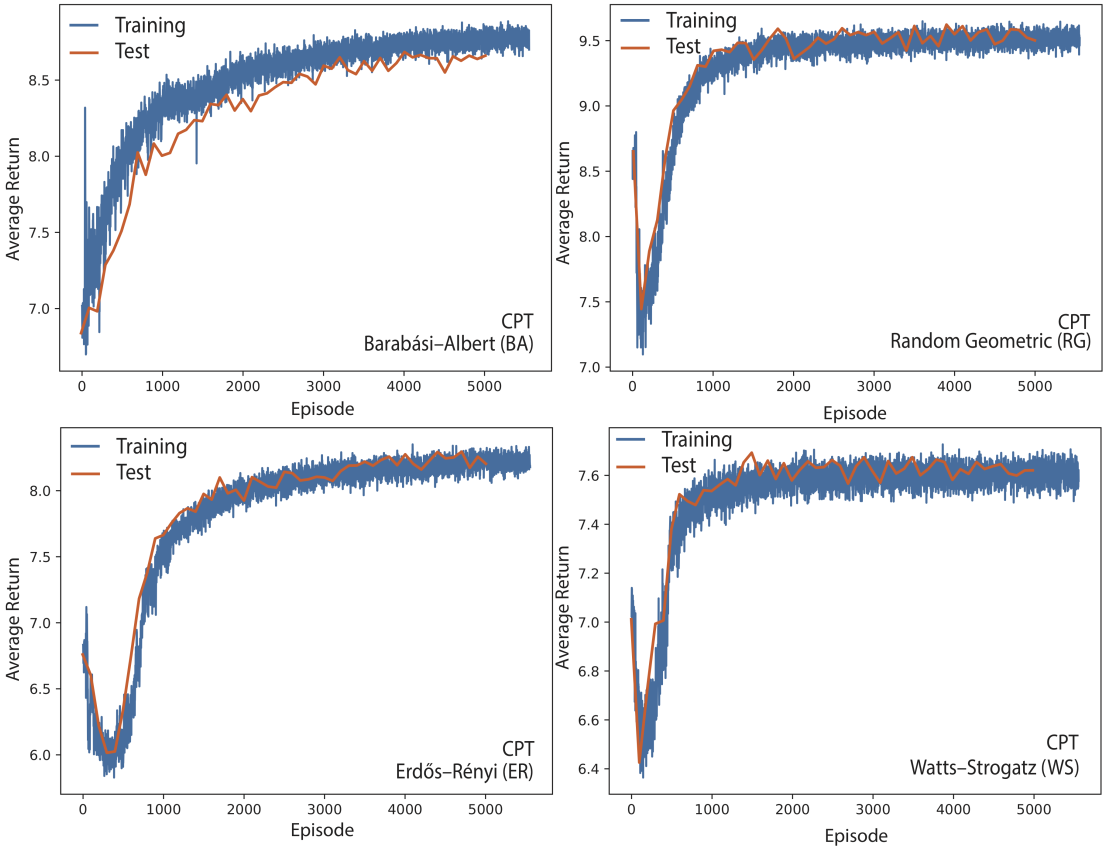


Figure S3: **Training and validation curves for compression progress theory.** We plot the training and validation performances of GNNs trained to optimize for network compressibility. Performance is measured as the average return. From left to right, top to bottom: (a) BA graphs, (b) RG graphs, (c) ER graphs, and (d) WS graphs. The results demonstrate generalization to the test set across several graph topologies.

# S3 Atlases

In Figure S4, we display a random geometric graph environment and plot atlases consisting of several trajectories on it produced by agents trained for the information gap and compression progress objectives. The two sets of trajectories are markedly different. The IGT agent navigates in a manner that produces several loops of edges. These loops, or topological cavities, are depicted in grey. The agent avoids creating triangles, as they would constitute higher dimensional simplices and might fill candidate cavities.

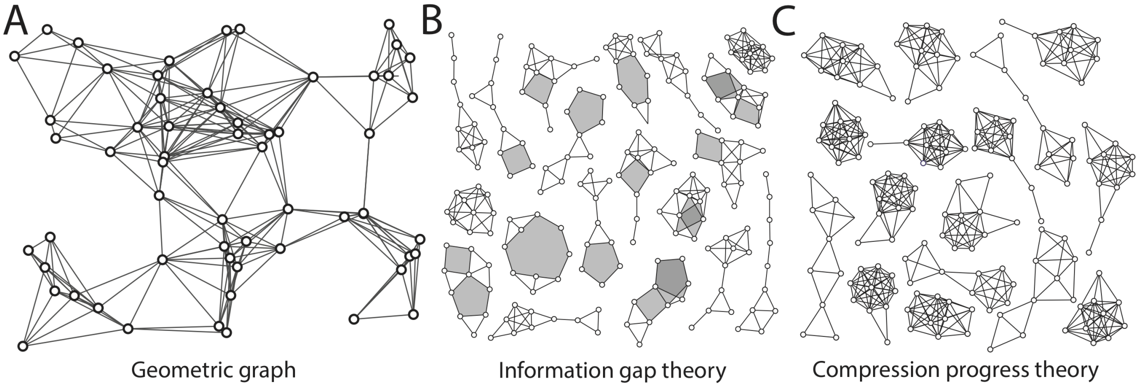


Figure S4: **Example of trajectories in a random geometric graph environment.** A) An instance of a random geometric graph environment. B) Examples of subgraphs produced by trajectories of 10 steps by a GNN agent trained for the IGT objective. Topological cavities in each trajectory are depicted in grey. C) Examples of subgraphs produced by trajectories of 10 steps by a GNN agent trained for the CPT objective.

The agent trained to optimize for network compressibility demonstrates a tendency to visit densely connected clusters of nodes. Clustering implies that neighbors of a node are also neighbors of each other. Therefore, in stark contrast to the IGT agent, trajectories produced by the CPT agent tend to have a high degree of triangular motifs. This visualization provides a compelling representation of the different policies learned by the two types of agents.

# S4 Trajectory length and network size generalization

In the experiments of the main text, we train GNN agents to take $10$ steps in environments of size $50$ nodes. Here, we show extended results about generalization to trajectories that are shorter and longer than $10$ steps, for all synthetic graph families. For these experiments, we keep the environment size fixed at 50 nodes. In Figure S5, we present results for agents trained for optimizing information gaps in each of the four synthetic graph models. Figure S6 depicts results for agents trained for the compression objective.

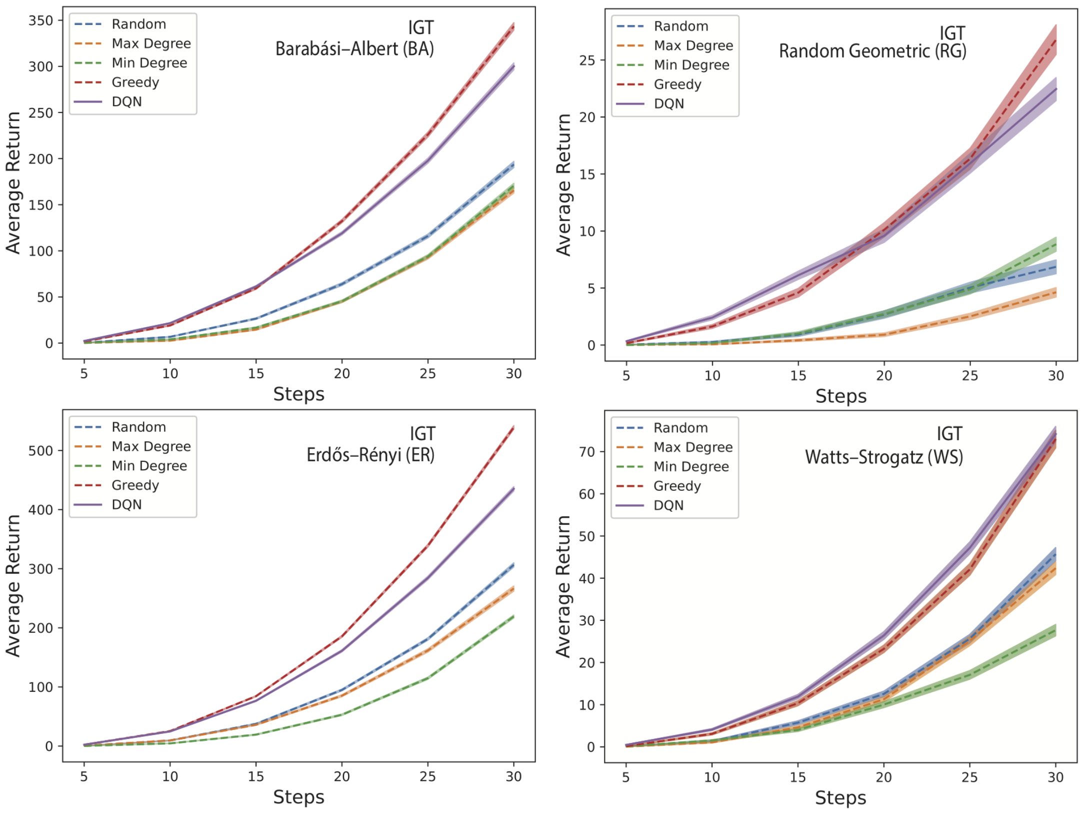


Figure S5: **Trajectory length generalization for information gap theory.** We train GNNs to explore for $10$ steps in graph environments with $50$ nodes. Here, we test generalization to walks of different lengths while holding the environment size fixed. From left to right, top to bottom, results for (a) BA graphs, (b) RG graphs, (c) ER graphs, and (d) WS graphs. The results demonstrate generalization to trajectories of different lengths than are seen during training.

In both sets of figures, the GNN agents consistently outperform the maximum degree, minimum degree, and random baselines. The GNN agents also closely match or outperform the greedy baseline. These findings highlight the effectiveness and reliability of the GNN-based approach in exploring graph-structured environments outside of the regimes in which training is conducted.

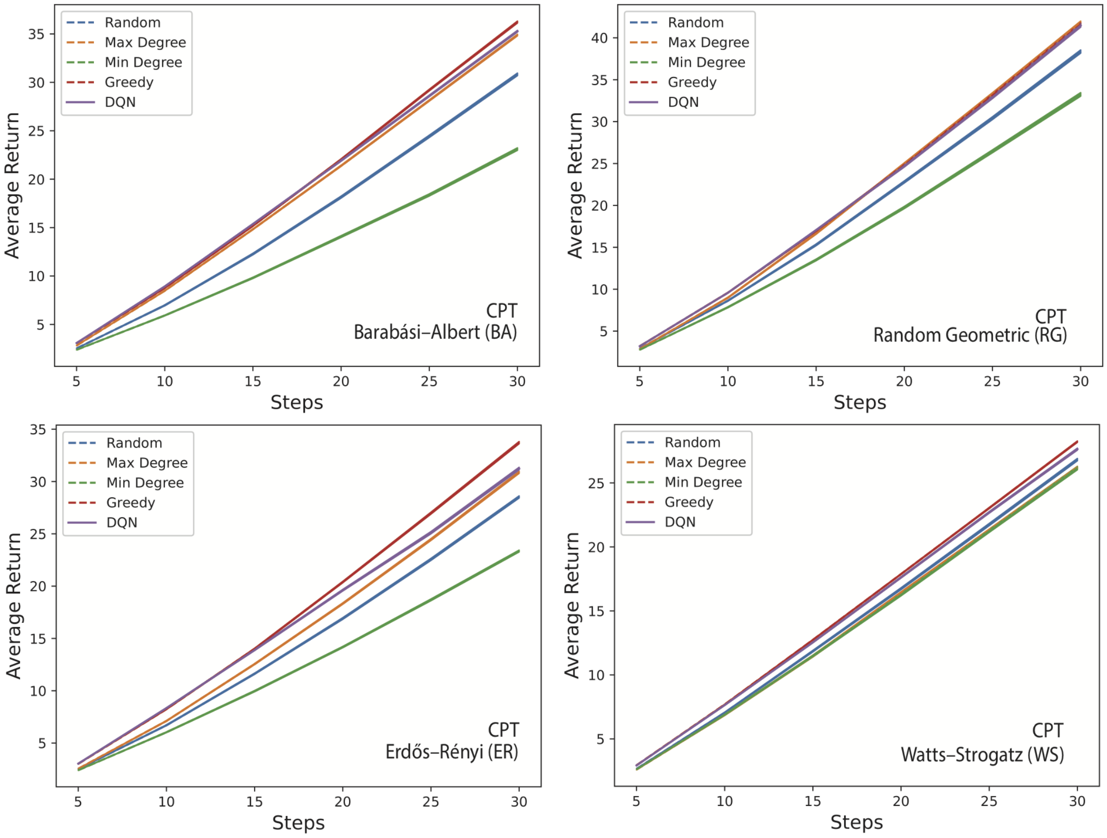


Figure S6: **Trajectory length generalization for compression progress theory.** We train GNNs to explore for 10 steps in graph environments with 50 nodes. Here, we test generalization to walks of different lengths while holding the environment size fixed. From left to right, top to bottom, results for (a) BA graphs, (b) RG graphs, (c) ER graphs, and (d) WS graphs. The results demonstrate generalization to trajectories of different lengths than are seen during training.

Local properties of networks do not always scale with network size. For instance, both degree distribution and clustering are graph features that have a dependency on the number of nodes. As a result, it is unclear whether policies learned for networks of one size will generalize effectively to networks of a different size. Therefore, after assessing generalizability for trajectory lengths, we next examine generalizability for environments of different sizes than are seen during training. In these experiments, we take 10 steps in environments that are either smaller or larger than 50 nodes.

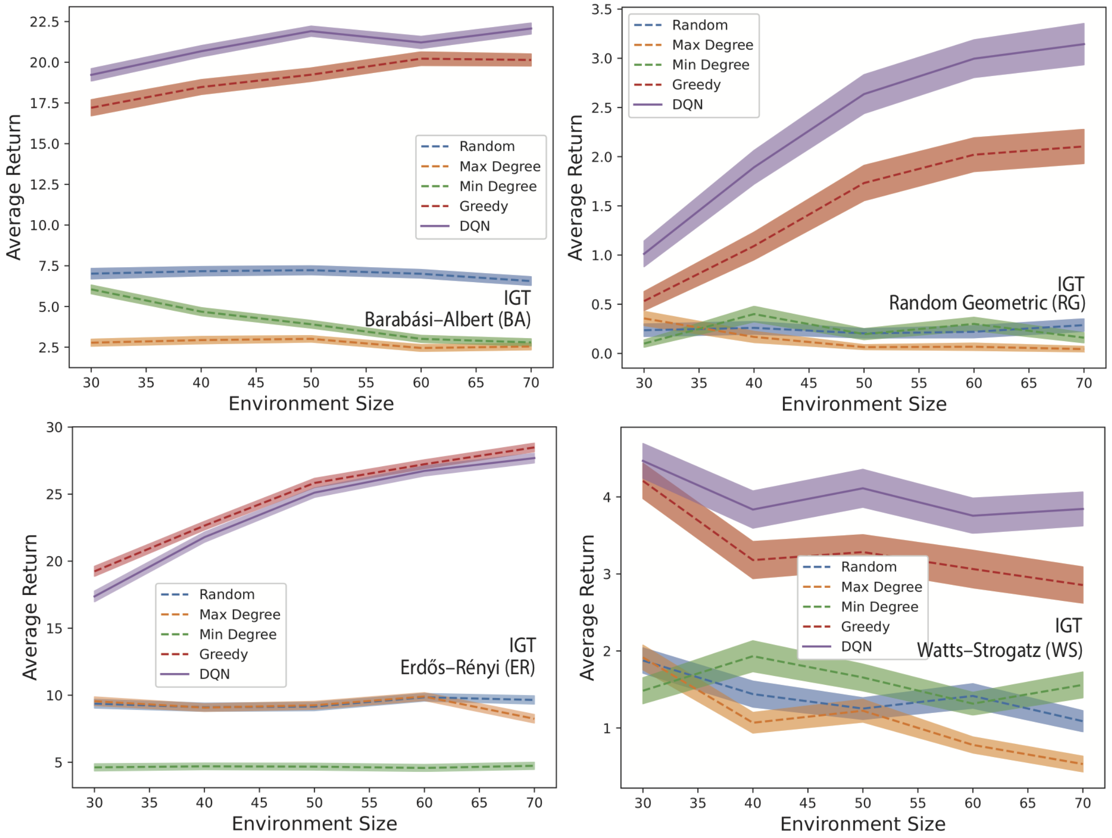


Figure S7: **Environment size generalization for information gap theory.** We train GNNs to explore for 10 steps in graph environments with 50 nodes. Here, we test generalization to environments of different sizes while holding the trajectory length fixed. From left to right, top to bottom, results for (a) BA graphs, (b) RG graphs, (c) ER graphs, and (d) WS graphs. The results demonstrate generalization to environments of different sizes than are seen during training.

Figure S7 depicts results for agents trained for information gap theory, while Figure S8 depicts results for compression progress theory. In both sets of figures, we find that the GNN agents outperform the maximum, minimum, and random baselines. They also perform at levels comparable to the one-step-ahead greedy evaluation of topological gaps and network compressibility.

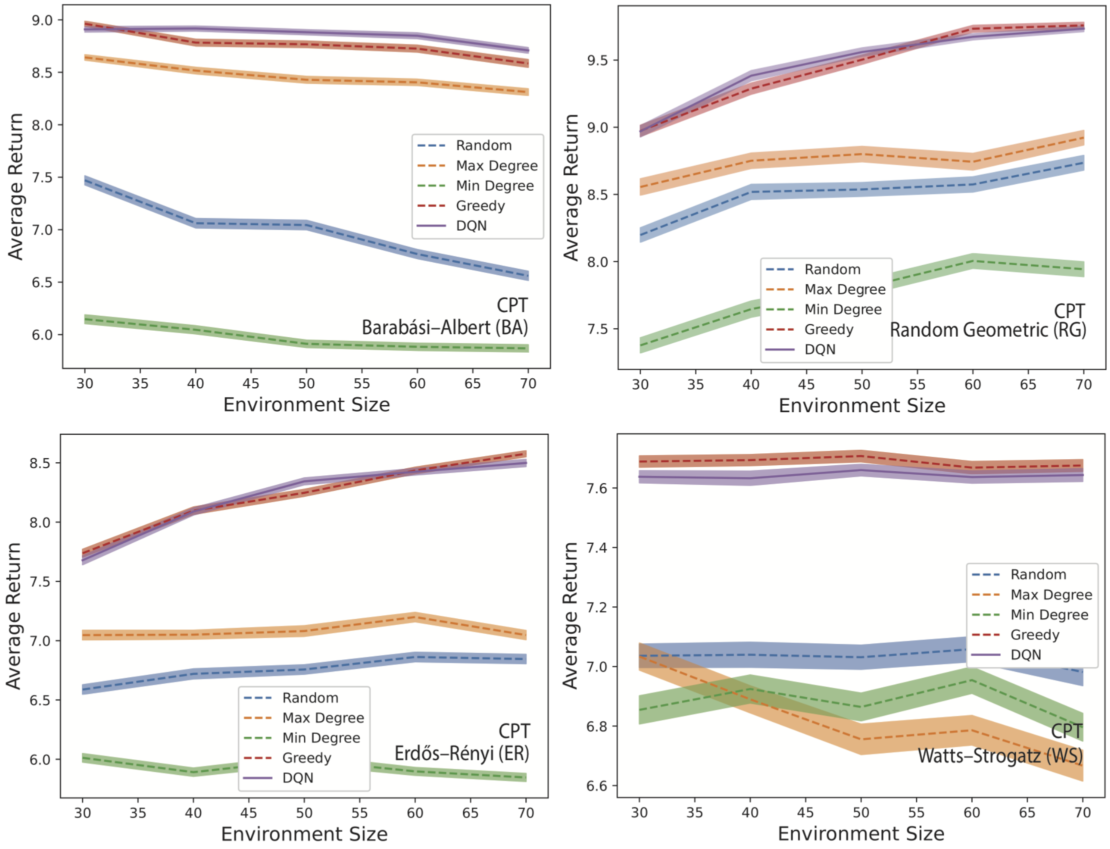


Figure S8: **Environment size generalization for compression progress theory.** We train GNNs to explore for 10 steps in graph environments with 50 nodes. Here, we test generalization to environments of different sizes while holding the trajectory length fixed. From left to right, top to bottom, results for (a) BA graphs, (b) RG graphs, (c) ER graphs, and (d) WS graphs. The results demonstrate generalization to environments of different sizes than are seen during training.

Our results from Figures S5, S6, S7, and S8 collectively indicate that GNNs for exploration can be trained in one set of circumstances and deployed in vastly different sets of circumstances.

## S5 Real-world graph datasets

We acquire trajectories of human graph exploration from three real-world datasets:

1. MovieLens: The MovieLens dataset contains sequences of movies watched by individual viewers alongside their associated reviews. [1]. We only keep movies that have at least five separate reviewers. We treat these movies as nodes and add edges between them based on the semantic similarity of their IMDb summaries. We construct vector embeddings for movies using a Word2Vec model pre-trained on the GoogleNews corpus [2]. We gather the first ten user-generated synopses available on IMDb for each movie and use cosine similarity to add edges to 20 other most similar movies. The resulting similarity network represents the graph environment for the GNN agent.
2. Amazon Books: The Amazon Product Reviews dataset contains sequential product purchase information by individual consumers for various categories of products [3, 4]. We limit our analyses to purchases of books. We filter out books with fewer than 150 reviews and only keep data for reviewers with at least 5 reviews. To represent each book as a distinct entity, we use Word2Vec-based vector embeddings. For each book, we add edges by identifying the top 20 most similar books based on their embeddings.
3. Wikispeedia: The Wikispeedia dataset consists of paths collected for a navigation game on Wikipedia [5, 6]. In the game, users are presented with a starting article and a destination article and are tasked with reaching the destination article using hyperlinks within Wikipedia. Here, the underlying hyperlink structure of Wikipedia acts as the graph environment.

The properties of the generated environments are summarized in the table below.

| | $N$ | $E$ | $\mid d \mid$ | $d_{min}$ | $d_{max}$ | $\rho$ | $\bar{l}_{path}$ |
|---|---|---|---|---|---|---|---|
| MovieLens | 1021 | 8143 | 15.96 | 1 | 105 | 0.015 | 8.45 |
| Amazon Books | 2115 | 38718 | 36.6 | 20 | 427 | 0.017 | 11.08 |
| Wikispeedia | 4592 | 106647 | 46.45 | 1 | 1621 | 0.01 | 9.12 |

Table S1: Summary information about MovieLens, Amazon Books, and Wikispeedia graph environments. We include the number of nodes ($N$), number of edges ($E$), average degree ($d$), minimum and maximum degree ($d_{min}$ and $d_{max}$), graph density ($\rho$), and the average length of trajectories ($l_{path}$) by exploring individuals. .

# S6 Random walker diffusion

A random walker biased according to compression progress theory (CPT) exhibits distinct diffusion behavior in the Wikispeedia network compared to the MovieLens and Amazon Books networks. On average, the CPT walker travels a shorter distance from the originating node in Wikispeedia, particularly after taking the second step. Network compressibility is strongly correlated with average clustering, which measures the propensity of a node's neighbors to be neighbors of each other [7]. Therefore, intuitively, greater clustering is reflected as more triangles in a network. To test whether Wikispeedia has unique clustering behavior, we sample sub-networks of different sizes by randomly picking a central node and expanding outwards according to a radius value.

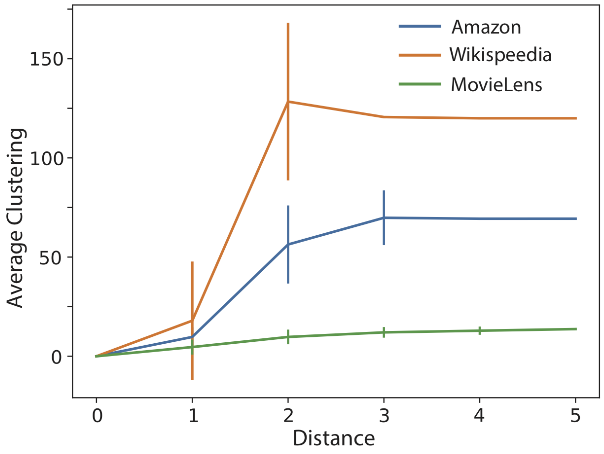


Figure S9: **Properties of the Real-world networks** Average number of triangles that nodes are involved in as a function of neighborhood radius.

In Figure S9, we plot the average number of triangular motifs that nodes participate in as a function of neighborhood radius. We find that Wikispeedia sub-networks have the greatest number of triangles when the neighborhood radius is two. Past this radius value, the average number of triangles that nodes participate in declines given the small-world nature of the Wikipedia graph [8]. Therefore, a walker seeking compression, or in other words, seeking greater clustering, usually has to go no further than two steps away from a starting point, as shown in Figure S9.

# S7 Human trajectories of graph exploration

In this section, we showcase several trajectories on the MovieLens network by a single individual. Given information about which movies this individual previously watched, we aim to predict the next movie. We contrast recommendations made by PageRank against those made by curiosity-biased PageRank. We highlight the user's actual next view in bold, showing that incorporating curiosity helps predict human behavior better.

Transition 1:
**Movies Previously Viewed:** *First Knight, The Little Mermaid, The Three Musketeers, Star Trek IV: The Voyage Home*
**Non-Biased:** *Titan A.E., Highlander, Dune, The Fifth Element, The Princess Bride, Beauty and the Beast*
**Biased:** *Army of Darkness, Highlander, Plan 9 from Outer Space, The Fifth Element, Arsenic and Old Lace,* **The Princess Bride**

Transition 2:
**Movies Previously Viewed:** *Star Trek IV: The Voyage Home, '2001: A Space Odyssey, Airplane!, Alien*
**Non-Biased:** *Con Air, Star Trek: The Motion Picture, Lost in Space, Titan A.E., Beneath the Planet of the Apes, Plan 9 from Outer Space*
**Biased:** *Beneath the Planet of the Apes, Sphere, Lost in Space,* **Aliens**, *Titan A.E., Plan 9 from Outer Space*

Transition 3:
**Movies Previously Viewed:** *Lock, Stock and Two Smoking Barrels, Honey, I Shrunk the Kids, Dead Poets Society, X2*
**Non-Biased:** *Fast Times at Ridgemont High, Rushmore, Thelma & Louise, Jumper, House of Wax, Charlie Bartlett*
**Biased:** *Jumper, Rushmore,* **The Fifth Element**, *Arsenic and Old Lace, Thelma & Louise, Charlie Bartlett*

Transition 4:
**Movies Previously Viewed:** *Demolition Man, Police Academy, Police Academy 2: Their First Assignment, Police Academy 3: Back in Training*
**Non-Biased:** *Porkys II: The Next Day, Police Academy 5: Assignment: Miami Beach,* **Police Academy 4: Citizens on Patrol**, *Police Academy 6: City Under Siege, S.W.A.T., The Enforcer*
**Biased:** *Collateral,* **Police Academy 4: Citizens on Patrol**, *Hot Fuzz, Sudden Impact, S.W.A.T., Porkys II: The Next Day*

# S8 Training details

## S8.1 Hyperparameters

We use the DQN algorithm to train GNNs for graph exploration [9]. The GNN architecture consists of $3$ rounds of GraphSAGE aggregation and combination [10]. The $5$ local degree profile (LDP) features (node degree, minimum and maximum degrees of neighbors, and the average and standard deviation of degrees of neighbors) are first embedded into $64$ dimensions over three rounds of GraphSAGE. Two fully-connected layers follow this, the first of which reduces dimensionality from $64$ to $32$, followed by a reduction to a single scalar Q-value in the final layer. We use a replay buffer to store experiences and a target network identical to the GNN to generate Q-value predictions. Training starts at step $320$ and continues for a total of $50000$ steps. Experiences are sampled from the buffer in batches of size $32$. The target network is updated every $16$ steps. We anneal the exploration rate $\epsilon$ linearly from $1$ to $0.1$ for the first $25000$ steps and then fix the rate at $0.1$ for the remainder of the training. We use a discount factor $\gamma$ of $0.75$ and use the Adam optimizer with a learning rate of $3 \times 10^{-4}$. These hyperparameters are summarized in the table below.

| **Parameter** | **Value** |
|---|---|
| Number of node features | 5 |
| GraphSAGE latent dimensions | 64 |
| FCN latent dimensions | 32 |
| Activation function | ReLU |
| Buffer size | 50000 |
| Training starts at step | 320 |
| Batch size | 32 |
| Transfer weights to target network ($C$) | every 16 steps |
| $\epsilon$ initial | 1 |
| $\epsilon$ smallest | 0.1 |
| Discount factor $\gamma$ | 0.75 |
| Optimizer | Adam |
| Learning rate | 3e-4 |

Next, we summarize the training algorithm.

## S8.2 Algorithm

**Algorithm 1** Deep Graph Q-learning with Experience Replay

Build featurized environment graph $\mathcal{G}$
Initialize replay buffer $\mathcal{D}$
Initialize neural network $\Phi(\cdot) : 2^{\mathcal{G}} \to \mathbb{R}$ with random weights $\Theta$
Initialize target network $\hat{\Phi}(\cdot) : 2^{\mathcal{G}} \to \mathbb{R}$ with weights $\hat{\Theta} = \Theta$
**for** episode = 1, M **do**
    Initialize list of visited nodes $\mathcal{V}_t = \{v_1\}$
    Build induced state subgraph $\mathcal{S}_t = \mathcal{G}[\mathcal{V}_t]$
    **for** t = 1, T **do**
        Get set of candidate next nodes $\mathcal{A}(\mathcal{S}_t) = \mathcal{N}(v_t) \backslash \mathcal{V}_t$
        **if** probability $< \epsilon$ **then**
            Select a random node $v_{t+1} \in \mathcal{A}(\mathcal{S}_t)$
        **else**
            Select $v_{t+1} = \max_a \Phi(\mathcal{S}_t, a; \Theta)$
        **end if**
        Set $\mathcal{S}_{t+1} = \mathcal{G}[\mathcal{V}_t \cup v_{t+1}]$
        Compute reward $R_t = \mathcal{F}(\mathcal{S}_{t+1})$
        Store transition $(\mathcal{S}_t, v_{t+1}, R_t, \mathcal{S}_{t+1})$ in $\mathcal{D}$
        Add $v_{t+1}$ to list of visited nodes $\mathcal{V}_t$
        Build induced state subgraph $\mathcal{S}_t = \mathcal{G}[\mathcal{V}_t]$
        Sample minibatch of transitions $(\mathcal{S}_j, v_{j+1}, R_j, \mathcal{S}_{j+1})$ from $\mathcal{D}$
        Set $y_j = \begin{cases} R_j, & \text{if } \mathcal{S}_{j+1} \text{ is terminal} \\ R_j + \gamma \max_{a'} \hat{\Phi}(\mathcal{S}_{j+1}, a'; \hat{\Theta}), & \text{otherwise} \end{cases}$
        If past burn-in, perform gradient descent to minimize $\mathbb{E}[y_j - \Phi(\mathcal{S}_j, v_{j+1})]^2$ and update $\Theta$
        Every $C$ steps, set $\hat{\Phi} \leftarrow \Phi$
    **end for**
**end for**

We use the same hyperparameters and training process for each synthetic and real-world graph dataset. The real-world datasets differ from the synthetic datasets in that there is no distinction between training, validation, and testing environments for the MovieLens, Amazon Books, and Wikispeedia networks, unlike the RG, WS, BA, and ER networks. We evaluate trained GNN agents in testing environments by removing $\epsilon$-greedy exploration and selecting actions greedily with respect to the Q-values.

## S9 Citation diversity statement

Recent work in a number of scientific fields has identified a bias in citation practices such that papers by women and other minority scholars are under-cited relative to the number of such papers in the field [11, 12, 13, 14, 15, 16, 17, 18, 19]. Here, we sought to proactively choose references that reflect the diversity of the field in thought, form of contribution, gender, race, ethnicity, and other factors. First, we predicted the gender of the first and last authors of each reference using databases that store the probability of a first name being carried by a woman [15, 20]. By this measure (and excluding self-citations to the first and last authors of our current paper), our references contain 3.61% woman(first)/woman(last), 8.25% man/woman, 14.13% woman/man, 74.01% man/man citation categorizations. This method is limited in that a) names, pronouns, and social media profiles used to construct the databases may not, in every case, indicate gender identity, and b) it cannot account for intersex, non-binary, or transgender people. Second, we obtained the predicted racial/ethnic category of the first and last author of each reference using databases that store the probability of a first and last name being carried by an author of color [21, 22]. By this measure (and excluding self-citations), our references contain 19.00% author of color/author of color, 13.97% white author/author of color, 21.38% author of color/white author, and 45.65% white author/white author citation categorizations. This method is limited in that a) names, Census entries, and Wikipedia profiles used to make predictions about gender may not be indicative of racial/ethnic identity, and b) it cannot account for Indigenous and mixed-race authors or those who may face differential biases due to the ambiguous racialization or ethnicization of their names. We look forward to future work that could help us to understand better how to support equitable practices in science.

## S10 References


[1] F Maxwell Harper and Joseph A Konstan. The movielens datasets: History and context. *Acm transactions on interactive intelligent systems (tiis)*, 5(4):1–19, 2015.

[2] Tomas Mikolov, Kai Chen, Greg S. Corrado, and Jeffrey Dean. Efficient estimation of word representations in vector space. *arXiv pre-print*, 2013. URL `http://arxiv.org/abs/1301.3781`.

[3] Ruining He and Julian McAuley. Ups and downs: Modeling the visual evolution of fashion trends with one-class collaborative filtering. In *proceedings of the 25th international conference on world wide web*, pages 507–517, 2016.

[4] Julian McAuley, Christopher Targett, Qinfeng Shi, and Anton Van Den Hengel. Image-based recommendations on styles and substitutes. In *Proceedings of the 38th international ACM SIGIR conference on research and development in information retrieval*, pages 43–52, 2015.

[5] Robert West and Jure Leskovec. Human wayfinding in information networks. In *Proceedings of the 21st international conference on World Wide Web*, pages 619–628, 2012.

[6] Robert West, Joelle Pineau, and Doina Precup. Wikispeedia: An online game for inferring semantic distances between concepts. In *Twenty-First International Joint Conference on Artificial Intelligence*, 2009.

[7] Christopher W. Lynn and Danielle S. Bassett. Quantifying the compressibility of complex networks. *Proceedings of the National Academy of Sciences*, 118(32):e2023473118, 2021. doi: 10.1073/pnas.2023473118. URL `https://www.pnas.org/doi/abs/10.1073/pnas.2023473118`.

[8] Myshkin Ingawale, Amitava Dutta, Rahul Roy, and Priya Seetharaman. The small worlds of Wikipedia: Implications for growth, quality and sustainability of collaborative knowledge networks. In *Proceedings of the 15th Americas Conference on Information Systems*, volume 5, page 439, 01 2009.

[9] Volodymyr Mnih, Koray Kavukcuoglu, David Silver, Andrei A. Rusu, Joel Veness, Marc G. Bellemare, Alex Graves, Martin Riedmiller, Andreas K. Fidjeland, Georg Ostrovski, Stig Petersen, Charles Beattie, Amir Sadik, Ioannis Antonoglou, Helen King, Dharshan Kumaran, Daan Wierstra, Shane Legg, and Demis Hassabis. Human-level control through deep reinforcement learning. *Nature*, 518(7540): 529–533, Feb 2015. ISSN 1476-4687. doi: 10.1038/nature14236. URL `https://doi.org/10.1038/nature14236`.

[10] William L. Hamilton, Rex Ying, and Jure Leskovec. Inductive representation learning on large graphs. In *Proceedings of the 31st International Conference on Neural Information Processing Systems*, NIPS'17, page 1025–1035, Red Hook, NY, USA, 2017. Curran Associates Inc. ISBN 9781510860964.

[11] Sara McLaughlin Mitchell, Samantha Lange, and Holly Brus. Gendered citation patterns in international relations journals. *International Studies Perspectives*, 14(4):485–492, 2013.

[12] Michelle L Dion, Jane Lawrence Sumner, and Sara McLaughlin Mitchell. Gendered citation patterns across political science and social science methodology fields. *Political Analysis*, 26(3):312–327, 2018.

[13] Neven Caplar, Sandro Tacchella, and Simon Birrer. Quantitative evaluation of gender bias in astronomical publications from citation counts. *Nature Astronomy*, 1(6):0141, 2017.

[14] Daniel Maliniak, Ryan Powers, and Barbara F Walter. The gender citation gap in international relations. *International Organization*, 67(4):889–922, 2013.

[15] Jordan D. Dworkin, Kristin A. Linn, Erin G. Teich, Perry Zurn, Russell T. Shinohara, and Danielle S. Bassett. The extent and drivers of gender imbalance in neuroscience reference lists. *bioRxiv*, 2020. doi: 10.1101/2020.01.03.894378. URL https://www.biorxiv.org/content/early/2020/01/11/2020.01.03.894378.

[16] Maxwell A. Bertolero, Jordan D. Dworkin, Sophia U. David, Claudia López Lloreda, Pragya Srivastava, Jennifer Stiso, Dale Zhou, Kafui Dzirasa, Damien A. Fair, Antonia N. Kaczkurkin, Bianca Jones Marlin, Daphna Shohamy, Lucina Q. Uddin, Perry Zurn, and Danielle S. Bassett. Racial and ethnic imbalance in neuroscience reference lists and intersections with gender. *bioRxiv*, 2020. doi: 10.1101/2020.10.12.336230.

[17] Xinyi Wang, Jordan D. Dworkin, Dale Zhou, Jennifer Stiso, Emily B Falk, Danielle S. Bassett, Perry Zurn, and David M. Lydon-Staley. Gendered citation practices in the field of communication. *Annals of the International Communication Association*, 2021. doi: 10.1080/23808985.2021.1960180.

[18] Paula Chatterjee and Rachel M Werner. Gender disparity in citations in high-impact journal articles. *JAMA Network Open*, 4(7):e2114509, 2021.

[19] Jacqueline M Fulvio, Ileri Akinnola, and Bradley R Postle. Gender (im)balance in citation practices in cognitive neuroscience. *J Cogn Neurosci*, 33(1):3–7, 2021.

[20] Dale Zhou, Eli J. Cornblath, Jennifer Stiso, Erin G. Teich, Jordan D. Dworkin, Ann S. Blevins, and Danielle S. Bassett. Gender diversity statement and code notebook v1.0, February 2020. URL https://doi.org/10.5281/zenodo.3672110.

[21] Anurag Ambekar, Charles Ward, Jahangir Mohammed, Swapna Male, and Steven Skiena. Name-ethnicity classification from open sources. In *Proceedings of the 15th ACM SIGKDD International Conference on Knowledge Discovery and Data Mining*, pages 49–58, 2009.

[22] Gaurav Sood and Suriyan Laohaprapanon. Predicting race and ethnicity from the sequence of characters in a name. *arXiv*, 2008.
